# Supplementary material for: Robust Output Regulation of Uncertain Linear Time-Varying Systems
Source: arXiv:2601.17464 source file (2026-08-26)
Supplement: Supplementary file 1 [file supplementary.pdf]

# Supplementary Information for Robust Output Regulation of Uncertain Linear Time-Varying Systems

Jinmeng Zha and Zhen Zhang

CONTENTS

**S1 Background** 2

**S2 Supplementary for Proposition 4.3** 3

**S3 Supplementary for Hypothesis 5.1** 4

**S4 Supplementary for Example 1** 5

**S5 Supplementary for Example 3** 6

Corresponding author: Z. Zhang (e-mail: zzhang@tsinghua.edu.cn). The authors are both with the Department of Mechanical Engineering, Tsinghua University, Beijing 100084, China.

## S1. Background

*Lie Derivative*: The Lie derivative is defined as

$$L_A^0 C(t) = C(t),$$
$$L_A^i C(t) = (L_A^{i-1} C(t))A(t) + \frac{\mathrm{d}}{\mathrm{d}t} L_A^{i-1} C(t),\ i \geq 1.$$

*Topologically Equivalent*: Two plant models are topologically equivalent if there exists a Lyapunov transformation to transform one into the other.

*Observability*: Consider the LTV plant $(A(t), B(t), C(t))$, its observability matrix is

$$\mathscr{O}_A(t) = \begin{bmatrix} L_A^0 C(t) \\ L_A^1 C(t) \\ \vdots \\ L_A^{r-1} C(t) \end{bmatrix}.$$

The observability Gramian is

$$W(t,s) = \int_t^s \Phi_A^T(\tau,t) C^T(\tau) C(\tau) \Phi_A(\tau,t)\,\mathrm{d}\tau.$$

The plant is *completely observable*, if for any $t \in \mathbb{R}$, there exists $s > t$ such that $W(t,s)$ is nonsingular. It is *uniformly completely observable*, if there exist constants $\alpha_1, \alpha_2, \delta > 0$, and a non-decreasing function $\gamma(t)$ such that for all $t, s \in \mathbb{R}$,

$$\alpha_1 I \leq W(t, t+\delta) \leq \alpha_2 I,\ ||\Phi_A(t,s)|| \leq \gamma(|t-s|).$$

*Neumann Series*: Suppose $||T|| < 1$ is a bounded operator on the normed vector space $X$. Then Neumann series indicates

$$(I-T)^{-1} = \sum_{k=0}^{\infty} T^k,$$

where $I$ is the identity operator.

*Multinomial Coefficient*: The multinomial theorem indicates

$$\left(\sum_{i=1}^m x_i\right)^n = \sum_{\substack{k_1+\cdots+k_m=n \\ k_1,\cdots k_m \geq 0}} \binom{n}{k_1, k_2, \cdots, k_m} x_1^{k_1} x_2^{k_2} \cdots x_m^{k_m},$$

where the multinomial coefficient is

$$\binom{n}{k_1, k_2, \cdots, k_m} = \frac{n!}{k_1! k_2! \cdots k_m!}.$$

## S2. Supplementary for Proposition 4.3

We omit arguments throughout this section. Calculations yield

$$\hat{A}_{\mathrm{cl}} = \begin{bmatrix} A_b + B_b K & B_b & & & \\ \alpha_1^T + \alpha_2 K - K(A_b + B_b K) & -k|b| + \alpha_2 + H_{\mathrm{im}} G_{\mathrm{im}} - K B_b & \alpha_3^T & -k|b|(-K\ 1)T_g^{-1} & bH_{\mathrm{im}} \\ (\beta\ 0) & & \eta & & \\ -g^{-(r-1)} B_b'(\alpha_1^T + \alpha_2 K) & -g^{-(r-1)} B_b'(-k|b| + \alpha_2 + H_{\mathrm{im}} G_{\mathrm{im}}) & -g^{-(r-1)} B_b' \alpha_3^T & gM_0 + g^{-(r-1)} B_b' k|b|(-K\ 1)T_g^{-1} & -g^{-(r-1)} B_b' b H_{\mathrm{im}} \\ -\frac{G_{\mathrm{im}}}{b}(\alpha_1^T + \alpha_2 K - K(A_b + B_b K)) & F_{\mathrm{im}} \frac{G_{\mathrm{im}}}{b} - \frac{\mathrm{d}}{\mathrm{d}t}\left(\frac{G_{\mathrm{im}}}{b}\right) - \frac{G_{\mathrm{im}}}{b}(\alpha_2 - K B_b) & -\frac{G_{\mathrm{im}}}{b} \alpha_3^T & & F_{\mathrm{im}} \end{bmatrix},$$

where $B_{\mathrm{b}}' \in \mathbb{R}^r$ is zeros except for the last element as 1; $\alpha^T(\cdot,\cdot) = [\alpha_1^T(\cdot,\cdot), \alpha_2(\cdot,\cdot), \alpha_3^T(\cdot,\cdot)]$, with $\alpha_1^T(\cdot,\cdot) \in \mathbb{R}^{r-1}, \alpha_2(\cdot,\cdot) \in \mathbb{R}, \alpha_3^T(\cdot,\cdot) \in \mathbb{R}^{n-r}$. Moreover, considering Young's inequality, namely

$$ab \leq \frac{ca^2}{2} + \frac{b^2}{2c},$$

for constants $a, b, c > 0$, it is calculated that

$$\begin{aligned} \hat{Q} = \mathrm{diag}\{ & c_1/2 - 2c_3\phi' a_2^2/a_3 - \phi'(c_5 a_2' \phi_G)^2 - 2, \\ & k\phi_b/4 - \phi'\gamma_1, \\ & c_3 a_3/2 - \phi'(c_5 a_2' \phi_G)^2 - 2, \\ & c_4 g - k\phi'[c_4 + (g^{r-1})^2 + (c_4 g^{-(r-1)})^2] - \phi'(c_4 g^{-(r-1)})^2 \gamma_2, \\ & c_5 a_3' - 5\}. \end{aligned}$$

## S3. SUPPLEMENTARY FOR HYPOTHESIS 5.1

*Proposition S3.1:* The family

$$\mathcal{F} = \left\{ b_\mu(t) = \frac{1}{b_0(t) + \mu E(t)} \,\middle|\, \mu \in \mathcal{P} \right\}$$

is infinite-dimensional if $E(\cdot) \neq c\, b_0(\cdot), \forall c \in \mathbb{R}$.

*Proof:* It suffices to show that the subset of functions corresponding to $\mathcal{P}' = \mathcal{P} \setminus \{\mathbf{0}\}$ spans an infinite-dimensional space. Rewrite $b_\mu(\cdot)$ as

$$b_\mu(t) = \frac{1}{b_0(t)} \frac{1}{1 + \mu b'(t)},$$

where $b'(t) = E(t)/b_0(t)$. Restrict attention to the interval $J_1$ where $b'(\cdot)$ is not a constant. Take any finite collection of distinct parameters $\mu_1, \cdots, \mu_n$ and suppose there exist constants $a_1, \cdots, a_n$ with $\sum_{i=1}^{n} a_i b_{\mu_i}(t) \equiv 0$, $t \in J_1$. Denote $J_2 = \mathrm{Im}(b'(t))$, $\forall t \in J_1$, and hence,

$$\sum_{i=1}^{n} a_i \frac{1}{1 + \mu_i x} \equiv 0, \quad x \in J_2.$$

Multiply it with $\prod_{j=1}^{n}(1 + \mu_j x)$ to obtain

$$P(x) = \sum_{i=1}^{n} a_i \prod_{j=1, j\neq i}^{n} (1 + \mu_j x) \equiv 0, \quad x \in J_2.$$

Because $P(x)$ is a polynomial, vanishing on an interval implies $P(x) \equiv 0$, $x \in \mathbb{R}$. Then for any $k = 1, \cdots, n$, we have $P(-1/\mu_k) = 0$, which means

$$a_k \prod_{j=1, j\neq k}^{n} (1 - \mu_j/\mu_k) = 0,$$

But $\{\mu_j\}$ is distinct, so $a_k = 0, k = 1, \cdots, n$. Therefore, any finite subcollection $\{b_{\mu_i}(t)\}$ is linearly independent. Because we can choose arbitrarily many distinct $\mu$-values in $\mathcal{P}'$, the set $\mathcal{F}$ contains arbitrarily large finite linearly independent subsets, so the linear span of $\mathcal{F}$ is infinite-dimensional. ■

## S4. Supplementary for Example 1

*Proposition S4.1:* The family $\mathcal{F}$ in Example 1, namely

$$\mathcal{F} = \left\{ \Omega_\mu(t) = \frac{\cos(t)}{(\sin(t) + 2 + \mu)^2} \,\middle|\, \mu \in [-0.5, 0.5] \right\}$$

is infinite-dimensional.

*Proof:* Restrict attention to the interval $J_1 = (-\Pi/2, \Pi/2)$. Take any finite collection of distinct parameters $\mu_1, \cdots, \mu_n$ and suppose there exist constants $a_1, \cdots, a_n$ with $\sum_{i=1}^n a_i \Omega_{\mu_i}(t) \equiv 0$, $t \in J_1$. Multiply it with $\prod_{j=1}^n (\sin(t) + 2 + \mu_j)^2$ to obtain

$$\cos(t) P(\sin(t)) \equiv 0, \quad t \in J_1, \tag{S1}$$

where

$$P(x) = \sum_{i=1}^n a_i \prod_{j=1, j\neq i}^n (x + 2 + \mu_j)^2,$$

Since $\cos(t) > 0$, $t \in J_1$, and $\sin(t)$ is a bijection from $J_1$ to $J_2 = (-1, 1)$, so (S1) is equivalent to $P(x) \equiv 0$, $x \in J_2$. Because $P(x)$ is a polynomial, vanishing on an interval implies $P(x) \equiv 0$, $x \in \mathbb{R}$. Then for any $k = 1, \cdots, n$, we have $P(-2 - \mu_k) = 0$, which means

$$a_k \prod_{j=1, j\neq k}^n (\mu_j - \mu_k)^2 = 0,$$

But $\{\mu_j\}$ is distinct, so $a_k = 0, k = 1, \cdots, n$. Therefore, any finite subcollection $\Omega_{\mu_i}(t)$ is linearly independent. Because we can choose arbitrarily many distinct $\mu$-values in $[-0.5, 0.5]$, the set $\mathcal{F}$ contains arbitrarily large finite linearly independent subsets, so the linear span of $\mathcal{F}$ is infinite-dimensional. ■

## S5. Supplementary for Example 3

*Proposition S5.1:* Recall Example 3 and fix $\varepsilon' = 1$. The family $\mathcal{F}$, namely

$$\mathcal{F} = \{R(t;\varepsilon) \mid \varepsilon \in [0.75, 1.25]\}$$

is infinite-dimensional.

*Proof:* Because $b, \mathscr{O}'_A(\mu)$ are constant and $\mathscr{O}'_S(t)$ is known, it suffices to show that the family

$$\mathcal{F}' = \left\{\Pi_1(t;\varepsilon) \mid \dot{\Pi}_1(t;\varepsilon) + \Pi_1(t;\varepsilon)S(t) = -\varepsilon\Pi_1(t;\varepsilon) + [\varepsilon' \; 1],\ \varepsilon \in [0.75, 1.25]\right\} \tag{S2}$$

is infinite-dimensional. Denote $\Pi_1(t;\varepsilon) = [p_1(t;\varepsilon), p_2(t;\varepsilon)]$, and substitute in (S2), obtaining that is suffices to show the family

$$\mathcal{F}'' = \left\{p_2(t;\varepsilon) \mid \ddot{p}_2 + 2\varepsilon\dot{p}_2 + [\varepsilon^2 + a + 2d(\cos(2t) + \cos(\sqrt{2}t))]p_2 = \varepsilon - \varepsilon',\ \varepsilon \in [0.75, 1.25] \setminus \{\varepsilon'\}\right\}$$

is infinite-dimensional. Denote $\Lambda = \{2m + \sqrt{2}n \mid m, n \in \mathbb{Z}\}$, and the solution admits the decomposition as followings

$$p_2(t;\varepsilon) = \sum_{\lambda\in\Lambda} c_\lambda(\varepsilon)e^{j\lambda t}.$$

Calculations yields

$$\mathbf{c}(\varepsilon) = (\mathbf{D}(\varepsilon) + d\mathbf{W})^{-1}\mathbf{b}(\varepsilon),$$

where $\mathbf{c}(\varepsilon) = \{c_\lambda(\varepsilon)\}_{\lambda\in\Lambda}$; $\mathbf{D}(\varepsilon)$ is a diagonal matrix with the diagonal element as $D_\lambda(\varepsilon) = (\varepsilon + j\lambda)^2 + a$; $\mathbf{W}$ is off-diagonal, defined as

$$\mathbf{W}_{\lambda,\lambda'} = \begin{cases} 1, & \text{if } (\lambda' - \lambda) \in \{\pm 2, \pm\sqrt{2}\}, \\ 0, & \text{otherwise;} \end{cases}$$

and $\mathbf{b}(\varepsilon)$ is zero except for $\mathbf{b}_0(\varepsilon) = \varepsilon - \varepsilon'$. Because $||\mathbf{D}^{-1}(\varepsilon)d\mathbf{W}|| < 1$, Neumann series yield

$$\mathbf{c}(\varepsilon) = \left(\sum_{k=0}^{\infty}(-1)^k d^k(\mathbf{D}^{-1}(\varepsilon)\mathbf{W})^k\right)\mathbf{b}'(\varepsilon),$$

where $\mathbf{b}'(\varepsilon)$ is zero except for $\mathbf{b}'_0(\varepsilon) = (\varepsilon - \varepsilon')/(\varepsilon^2 + a)$. Moreover,

$$\mathbf{c}_{2m}(\varepsilon) \sim O\left(\frac{1}{\varepsilon^{2m+1}}\right),\ m \in \mathbb{Z}.$$

Because a set of rational functions with strictly distinct denominator degrees is linearly independent, the family of solution vectors $\{\mathbf{c}(\varepsilon)\}$ spans an infinite-dimensional space. Therefore, $\mathcal{F}''$ is infinite-dimensional, completing the proof. ■
